# Supplementary material for: A comparative study of micromorphic gradient-extensions for anisotropic damage at finite strains
Source: arXiv:2311.15918 source file (2023-11-27)
Supplement: Supplementary file 1 [file appendix.tex]

\clearpage

\appendix

\section{Appendix}
\label{sec:appendix}

\begin{figure}[htbp]
    \missingfigure{ANotched: Damage Plot mat124 mit A=1000? -> Gerader Schubriss statt S-Form (inkl. Netzverkonvergenz vorhanden)}
\end{figure}

\begin{figure}[htbp]
    \missingfigure{ANotched: Damage Plot mat128 -> ``falsche'' entwicklung von Dyy an notch}
\end{figure}

%----------------------------------------------------------------------------------------------------------------------------------%
\subsection{Appendix 1}
\label{sec:app_1}

appendix a 1

\subsection{Appendix 2}
\label{sec:app_2}

appendix a 2
